# Supplementary material for: UQSA -- An R-Package for Uncertainty Quantification and Sensitivity Analysis for Biochemical Reaction Network Models
Source: arXiv:2308.05527 source file (2026-09-19)
Supplement: Supplementary file 1 [file supplementary.tex]

\documentclass[DIV=14, english]{scrartcl}
\pdfoutput=1
\usepackage[utf8]{inputenc}
\usepackage{lmodern}
\usepackage{FiraSans}
\usepackage[T1]{fontenc}
\usepackage{amsmath,amssymb}
\usepackage{graphicx}
\usepackage{authblk}
\usepackage{microtype}
\usepackage{babel}
\usepackage{multicol}
\usepackage{enumitem}
\usepackage[normalem]{ulem}
\usepackage{siunitx}
\usepackage{booktabs}
\usepackage[dvipsnames]{xcolor}
\usepackage{url}
\usepackage[version=4]{mhchem}
% \usepackage[%
%  colorlinks=true,%
%  linkcolor=blue!20!black,%
%  citecolor=green!20!black,%
%  urlcolor=magenta!20!black%
%  ]{hyperref}
% Make the Section numbers line up with upper case letters:
\addtokomafont{section}{\firalining}
\addtokomafont{subsection}{\firalining}

%\access{Advance Access Publication Date: Day Month Year}
%\appnotes{Manuscript Category}
\usepackage{soul}
% this makes "Figure N" in captions bold, and the next line not be indented
\setcapindent{0pt}
\addtokomafont{captionlabel}{\bfseries}

%\firstpage{1}

%\subtitle{Systems biology}

%\subject{{\sffamily\Large Systems Biology and Neuroscience}}
\subject{Supplementary material}
\title{UQSA - an R-package for Bayesian uncertainty quantification and global sensitivity analysis for biochemical reaction network models }

\date{}

\author[$1$,+,*]{Andrei Kramer}
\author[$2$,+]{Federica Milinanni}
\author[$3$] {Jeanette Hellgren Kotaleski}
\author[$2$, $4$]{Pierre Nyquist}
\author[$5$,o]{Alexandra Jauhiainen}
\author[$3$,o,*]{Olivia Eriksson}

%\author{Andrei Kramer\, Federica Milinanni\,$^{\text{\sfb 2,+}}$ Pierre Nyquist\,$^{\text{\sfb 2,}}$ \\
%Alexandra Jauhiainen\,$^{\text{\sfb 3,o}}$ and Olivia Eriksson$^{\text{\sfb 4,o,*}}$}

\affil[$1$] {Science for Life Laboratory, Department of Neuroscience, Karolinska Institute, Solna, Sweden}
\affil[$2$] {Department of Mathematics, KTH Royal Institute of Technology, Stockholm, Sweden.}
\affil[$3$] {Science for Life Laboratory, School of Electrical Engineering and Computer Science, KTH Royal Institute of Technology, Sweden}
\affil[$4$] {Department of Mathematical Sciences, Chalmers University of Technology and University of Gothenburg, Gothenburg, Sweden.}
\affil[$5$] {R\&I Biometrics and Statistical Innovation, Late Respiratory \& Immunology, BioPharmaceuticals R\&D, AstraZeneca, Gothenburg, Sweden}

\affil[*] {To whom correspondence should be addressed.}
\affil[+] {Have contributed equally to this work as first authors.}
\affil[o] {Have contributed equally to this work as last authors.}

\begin{document}
\maketitle

\begin{abstract}
  In this supplementary material we show what kind of output the
  package produces and provide some guidance on which sampling
  algorithm to chose. We compare their performance for one medium
  sized model. There are dedicated publications on scaling and
  performance benchmarking between different toolboxes/packages, which
  is outside of the scope of this manuscript. We use the standard
  tools and concepts of the field for benchmarking.
\end{abstract}

Figure~\ref{fig1S} illustrates the general idea behind sampling for
parameter estimation and predictions with Bayesian uncertainty
quantification and global sensitivity analysis. It shows the propagation of uncertainty in the model and data to the prediction and sensitivity analysis. 

The sampling algorithms in this package produce posterior distribution
samples, which are typically represented as pairwise matrix plots of
all two dimensional projections, as shown in Figure~\ref{fig:AKAP79-4}
(restricted to 4 out of the 27 parameters). In some cases parallel
coordinate plots may also work well. The model we chose for
illustration purposes has parameter names that include the reacting
species in their names, so rather than $k_{\text{f},1}$ we use a name
like $k^{\text{f}}_{\ce{A + B \to C}}$ or \texttt{kf\_A\_B\_\_C}. It is included with the package as an example model: \texttt{AKAP79}.

\begin{figure*}
\centering
\includegraphics[width=\textwidth]{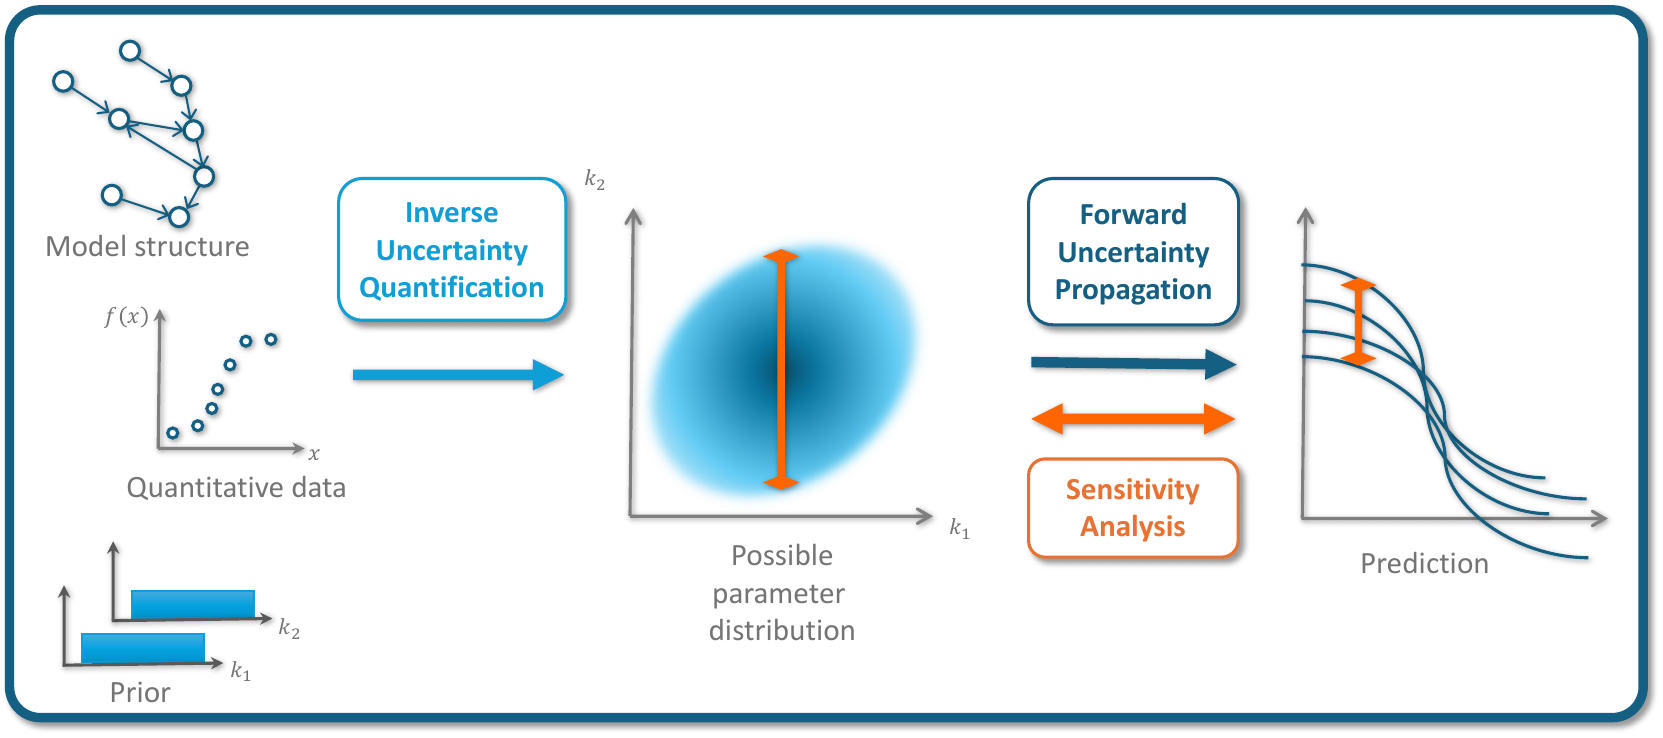}
\caption{\footnotesize Full model calibration requires to quantify the
  uncertainty of the parameter estimates through a Bayesian approach
  (\textcolor{Blue}{inverse uncertainty quantification}) and to
  propagate this uncertainty (the posterior distribution) to the
  predictions made from the model (\textcolor{Blue}{forward
    uncertainty propagation}). Finally a global sensitivity analysis
  can be performed on the posterior distribution to guide further
  experiments (\textcolor{RedOrange}{sensitivity analysis}). Figure
  adapted from \cite{eriksson2019uncertainty}.}\label{fig1S}
\end{figure*}

\begin{figure}
  \centering
  \includegraphics[width=\textwidth]{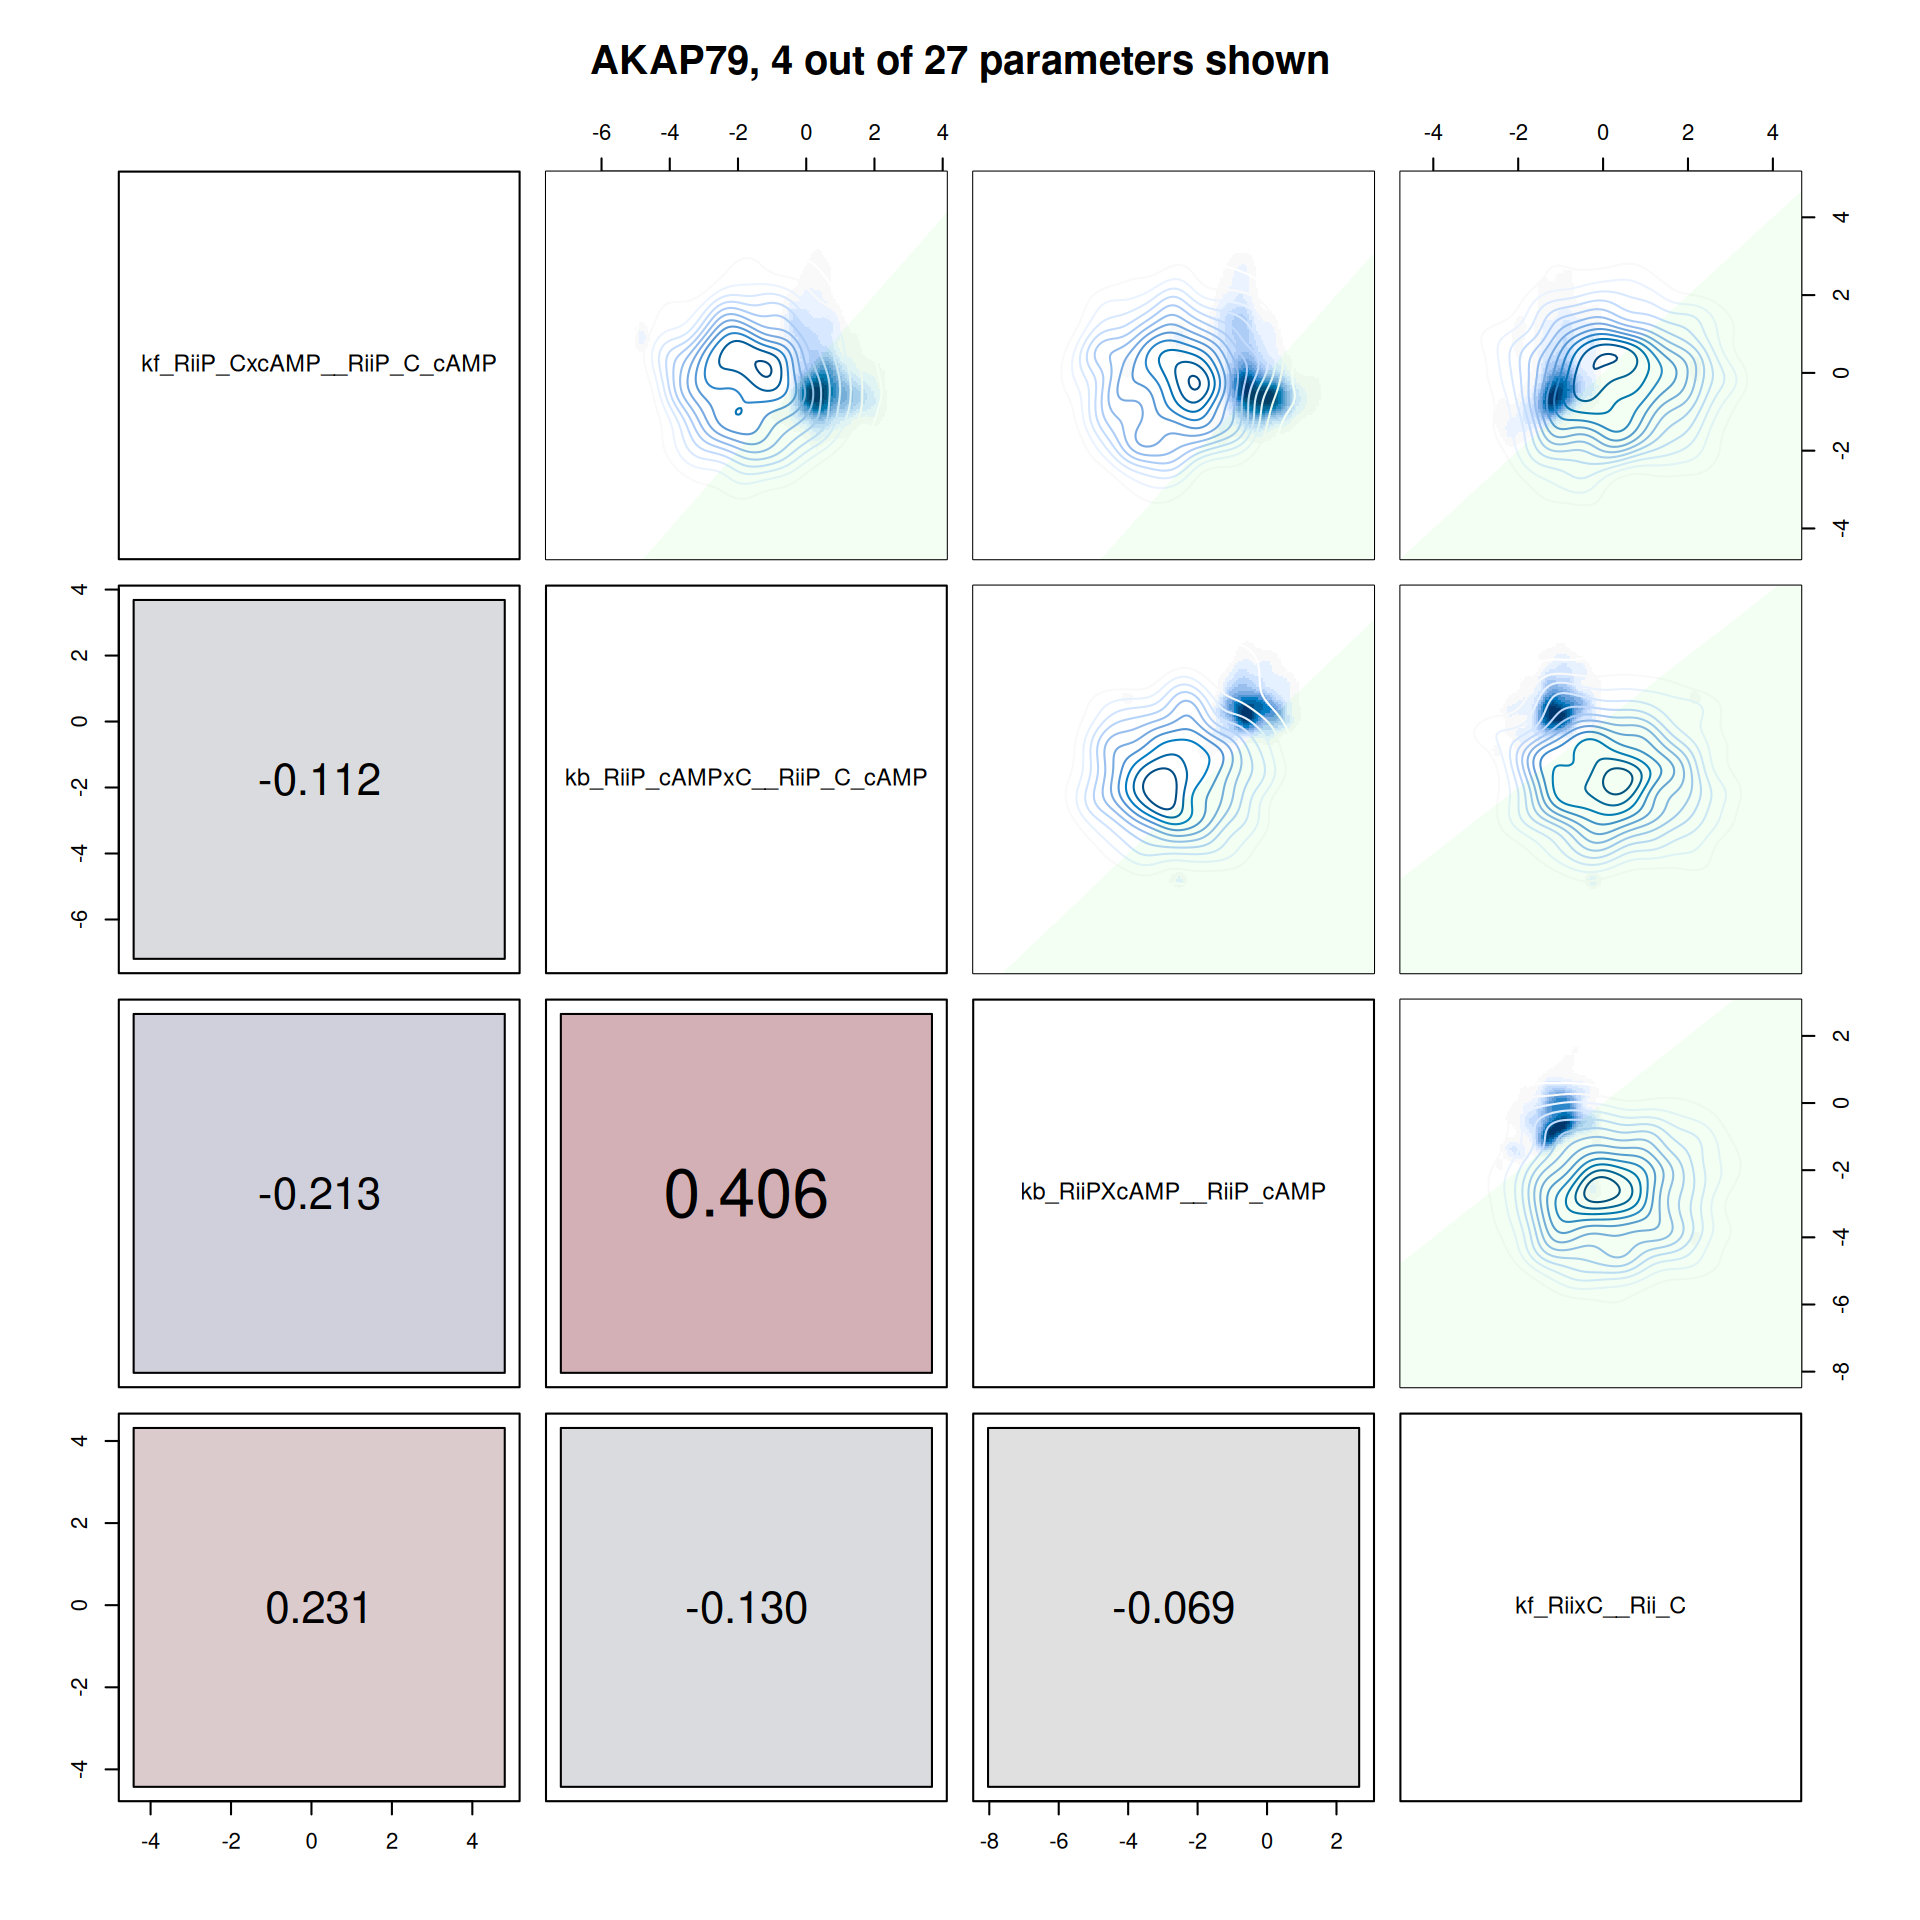}
  \caption{The sample obtained with PT SMMALA on PDC (hpc cluster
    located at KTH), shown as pairs of two dimensional projections. We
    picked 4 out of the 27 parameters for visibility. The upper panels
    show the posterior distribution via shading and the prior using
    contour lines (level sets). If the prior and posterior are too
    similar, the lines blend in with the shading. Otherwise the lines
    are clearly visible, because the posterior and prior are very
    different. We use the sample of the lowest inverse temperature
    $\beta \ll 1$ as proxy for the prior (it is a very good
    approximation). The shaded posterior distribution is more
    concentrated (smaller covariance), i.e. we inferred a lot of
    information about the parameters from the data. Areas shaded green
    are below the identity line ($x = y$), which is useful to identify
    or confirm possible inequalities (or inequality constraints). The
    lower panels show the correlation of the posterior (with colors
    and numbers).\label{fig:AKAP79-4}}
\end{figure}

Figure~\ref{fig:AKAP79-8-9} shows one of these panels, and also one
dimensional representations of the posterior and prior as
histograms. Figure~\ref{fig:AKAP79-state-func-gsa} shows a different pair
of parameters and trajectories of the model from one of the
experiments (\qty{2}{\nano\mole\per\litre} cAMP and \qty{0}{\nano\mole\per\litre} CaN in the AKAP79 model). We display the observable
\texttt{AKAP4p} (data with errorbars) and one of the state variables
which was not measured during the experiment (no data, a prediction). Figure~\ref{fig:AKAP79-state-func-gsa} shows the first order Sobol sensitivity indices, and which parameter that if known would reduce the uncertainty in \texttt{AKAP4p} the most. 

\begin{figure}
  \centering
  \includegraphics[width=\textwidth]{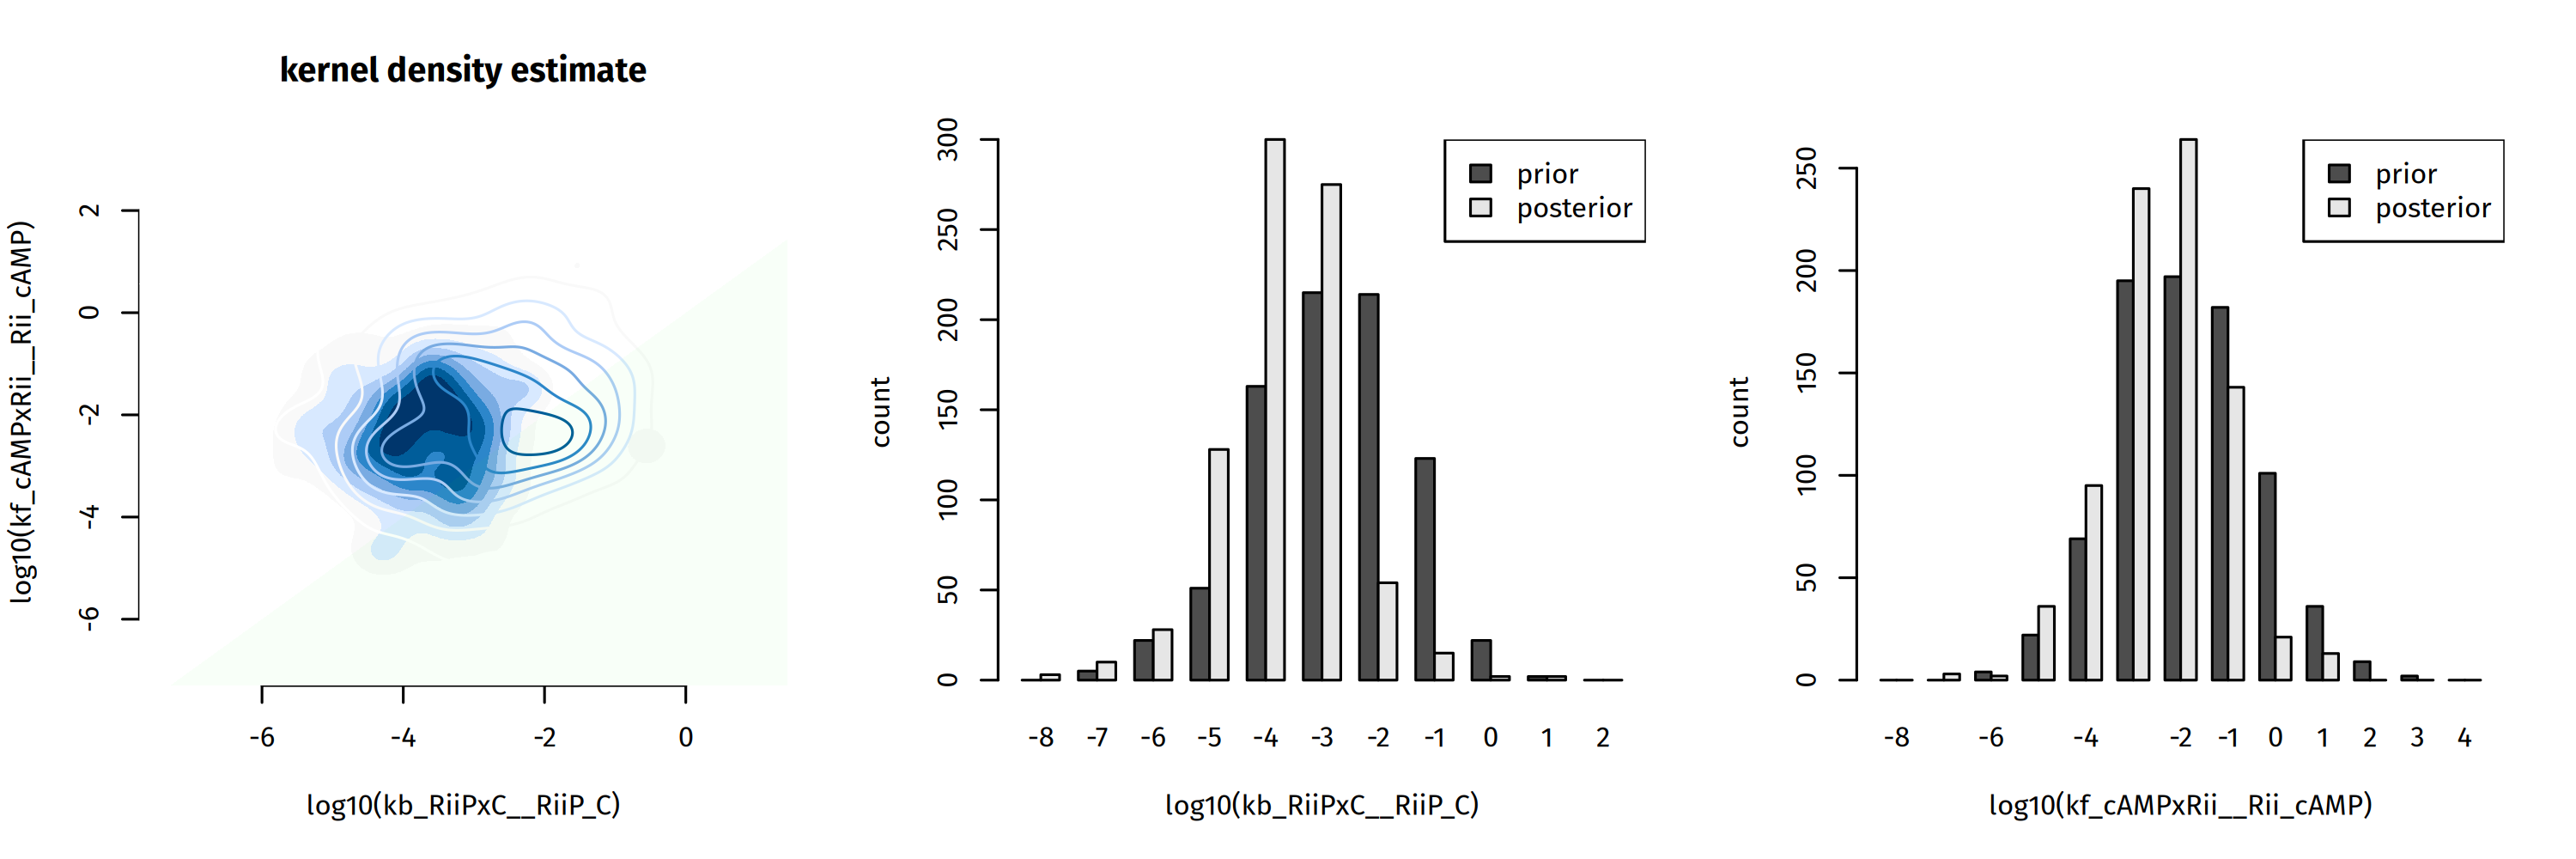}
  \caption{Here we show one two dimensional projection between
    parameters 8 and 9 and also the one dimensional projection of both
    as histograms. The two dimensional plots make the differences
    between posterior and prior much more apparent.\label{fig:AKAP79-8-9}}
\end{figure}

To give the user an idea about which algorithm to use, we ran a benchmark on the PDC cluster at KTH. We used one
node\footnote{to sample the problem really thoroughly, we would use more nodes and more time -- 1 node and 1 to 3 hours of sampling time (wall clock time) is enough to estimate the sampling speed for a model of this size} with 128 cores and gave each algorithm a workload for
approximately one hour. A different model may be harder or easier to sample for any of the algorithms, but Table~\ref{tab:benchmark} describes a typical performance pattern for systems biology models. Algorithms with low sampling speed have redeeming qualities: they can be easier to use (ABC and RWM) because they require less model prerequisites\footnote{SMMALA needs the likelihood's gradient, and Fisher information}. For most stochastic models, ABC is one of the most important sampling methods, that works reliably.

The ABC algorithm (Approximate Bayesian Computation) is somewhat different from the other MCMC
algorithms. We embed the deterministic ODE solution into a random
process that emulates measurement noise. The likelihood-based algorithms all use the deterministic (numerical) ODE solutions without added noise\footnote{this has very little impact on performance}. ABC can also be used with intrinsically stochastic models (with Gillespie algorithm solvers) where likelihood based methods are unavailable.

One major question is whether or not to use parallel tempering
(PT). Even without any implemented strategy, a cluster can be used to
obtain several replica of the posterior sample in parallel (using
different pseudo random number sequences). This trivially increases
the final sample size (but doesn't help with convergence to the target
distribution).

With parallel tempering the auto-correlation is smaller: better
sample quality, faster mixing/convergence. But PT creates two
overheads:
\begin{enumerate}
\item communication between the chains, requires all chains to wait
  until they are synchronized in their workload:
  \begin{itemize}
  \item We used the setting that attempts to swap between two chains
    on every iteration of the MCMC algorithm.
  \item Trivially parallel algorithms do not communicate and never
    pause to synchronize.
  \end{itemize}
\item chains running on an inverse temperature of $0 < \beta < 1$ sample from a
  relaxed problem and not from the posterior
  \begin{itemize}
  \item They are effectively \emph{helper chains}.
  \item They do not contribute to the sample size, only $\beta=1$ does.
  \item The returned sample is smaller, but of higher quality.
  \end{itemize}
\end{enumerate}

Given a good estimate for the likelihoods integrated auto-correlation
length\footnote{In $\tau_{l,\dots}$ the $l$ indicates that we use the
  log-likelihood values of the sample to calculate $\tau$}
$\tau_{l,\text{int.}}$, we can calculate an \emph{effective sample
  size}, which takes the sample's quality into account.

We further divide this value by the consumed wall-clock time $w$:
\begin{equation}
  \label{eq:samplingspeed}
  v = \frac{N}{2 \tau_{l,\text{int.}} w}\,,
\end{equation}
which is our final estimate of \emph{performance} (the scheduled
compute resources were identical). We use the R package
\texttt{hadron}\footnote{\url{https://github.com/HISKP-LQCD/hadron}}
to estimate the auto-correlation in this benchmark. The effectively
sampling speeds are summarized in Table~\ref{tab:benchmark}. We use
concise error notation: $0.09(1)\times 10^3$ is
$(0.09 \pm 0.01)\times 10^3$ in common terms.

We have used parallel tempering in two ways
\begin{itemize}
\item 128 MPI workers, and 128 temperatures:
  \begin{itemize}
  \item each worker has their own $0 < \beta \le 1$ value
  \item many temperatures (as many as possible)
  \item highest possible sample quality
  \item smallest returned raw sample size $N$ (from one MPI worker)
  \end{itemize}
\item 128 MPI workers, but 16 temperatures
  \begin{itemize}
  \item repeating the same temperature several times
  \item reasonable number of temperatures
  \item compromise between sample size and sample quality
  \item bigger raw sample size $N$ (from 8 MPI workers)
  \end{itemize}
\end{itemize}

The benchmark illustrates that it stops being beneficial to add more
inverse temperatures and it is more useful to have several workers
operate at $\beta = 1$ (the unrelaxed posterior distribution). This
increases the raw sample size and uses the compute resources more
efficiently.

\begin{figure}
  \centering
  \includegraphics[width=\textwidth]{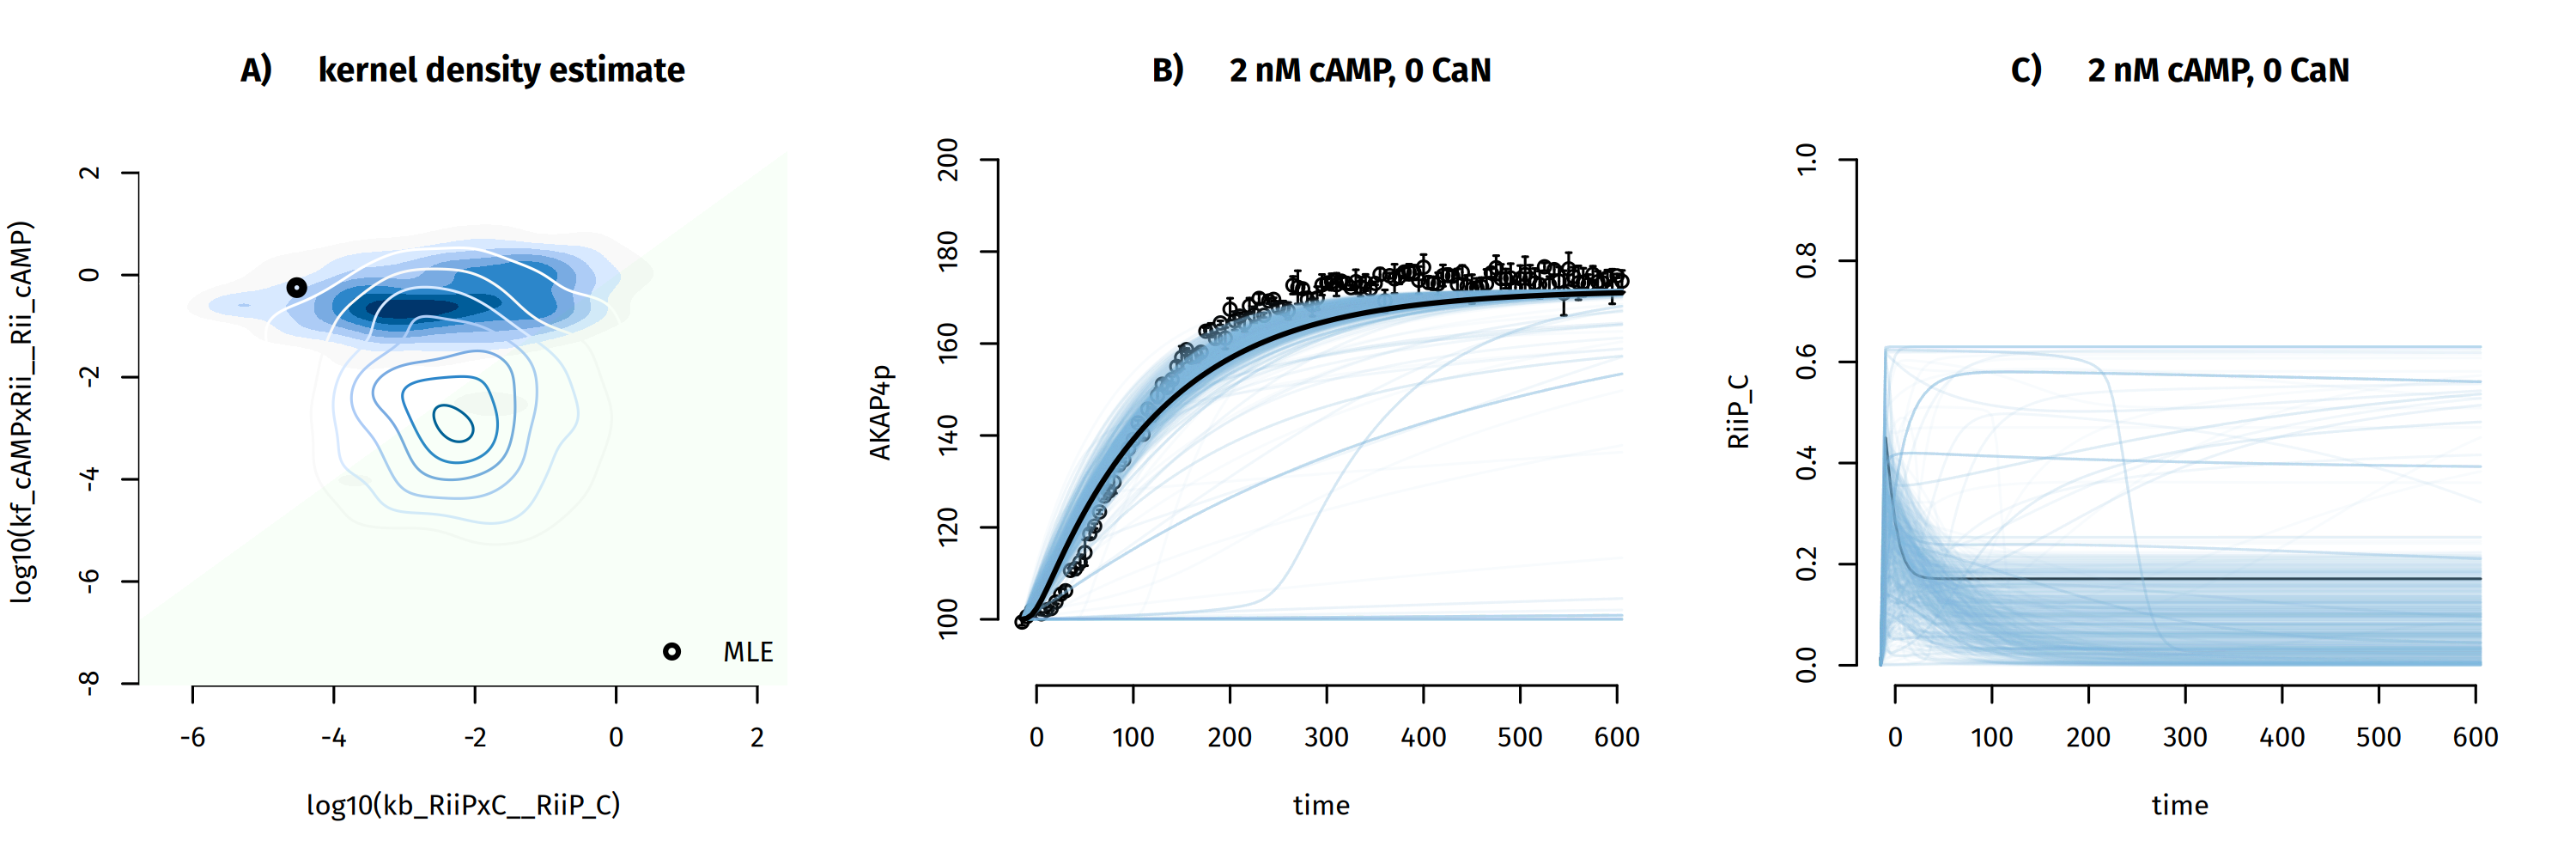}\\
  \includegraphics[width=\textwidth]{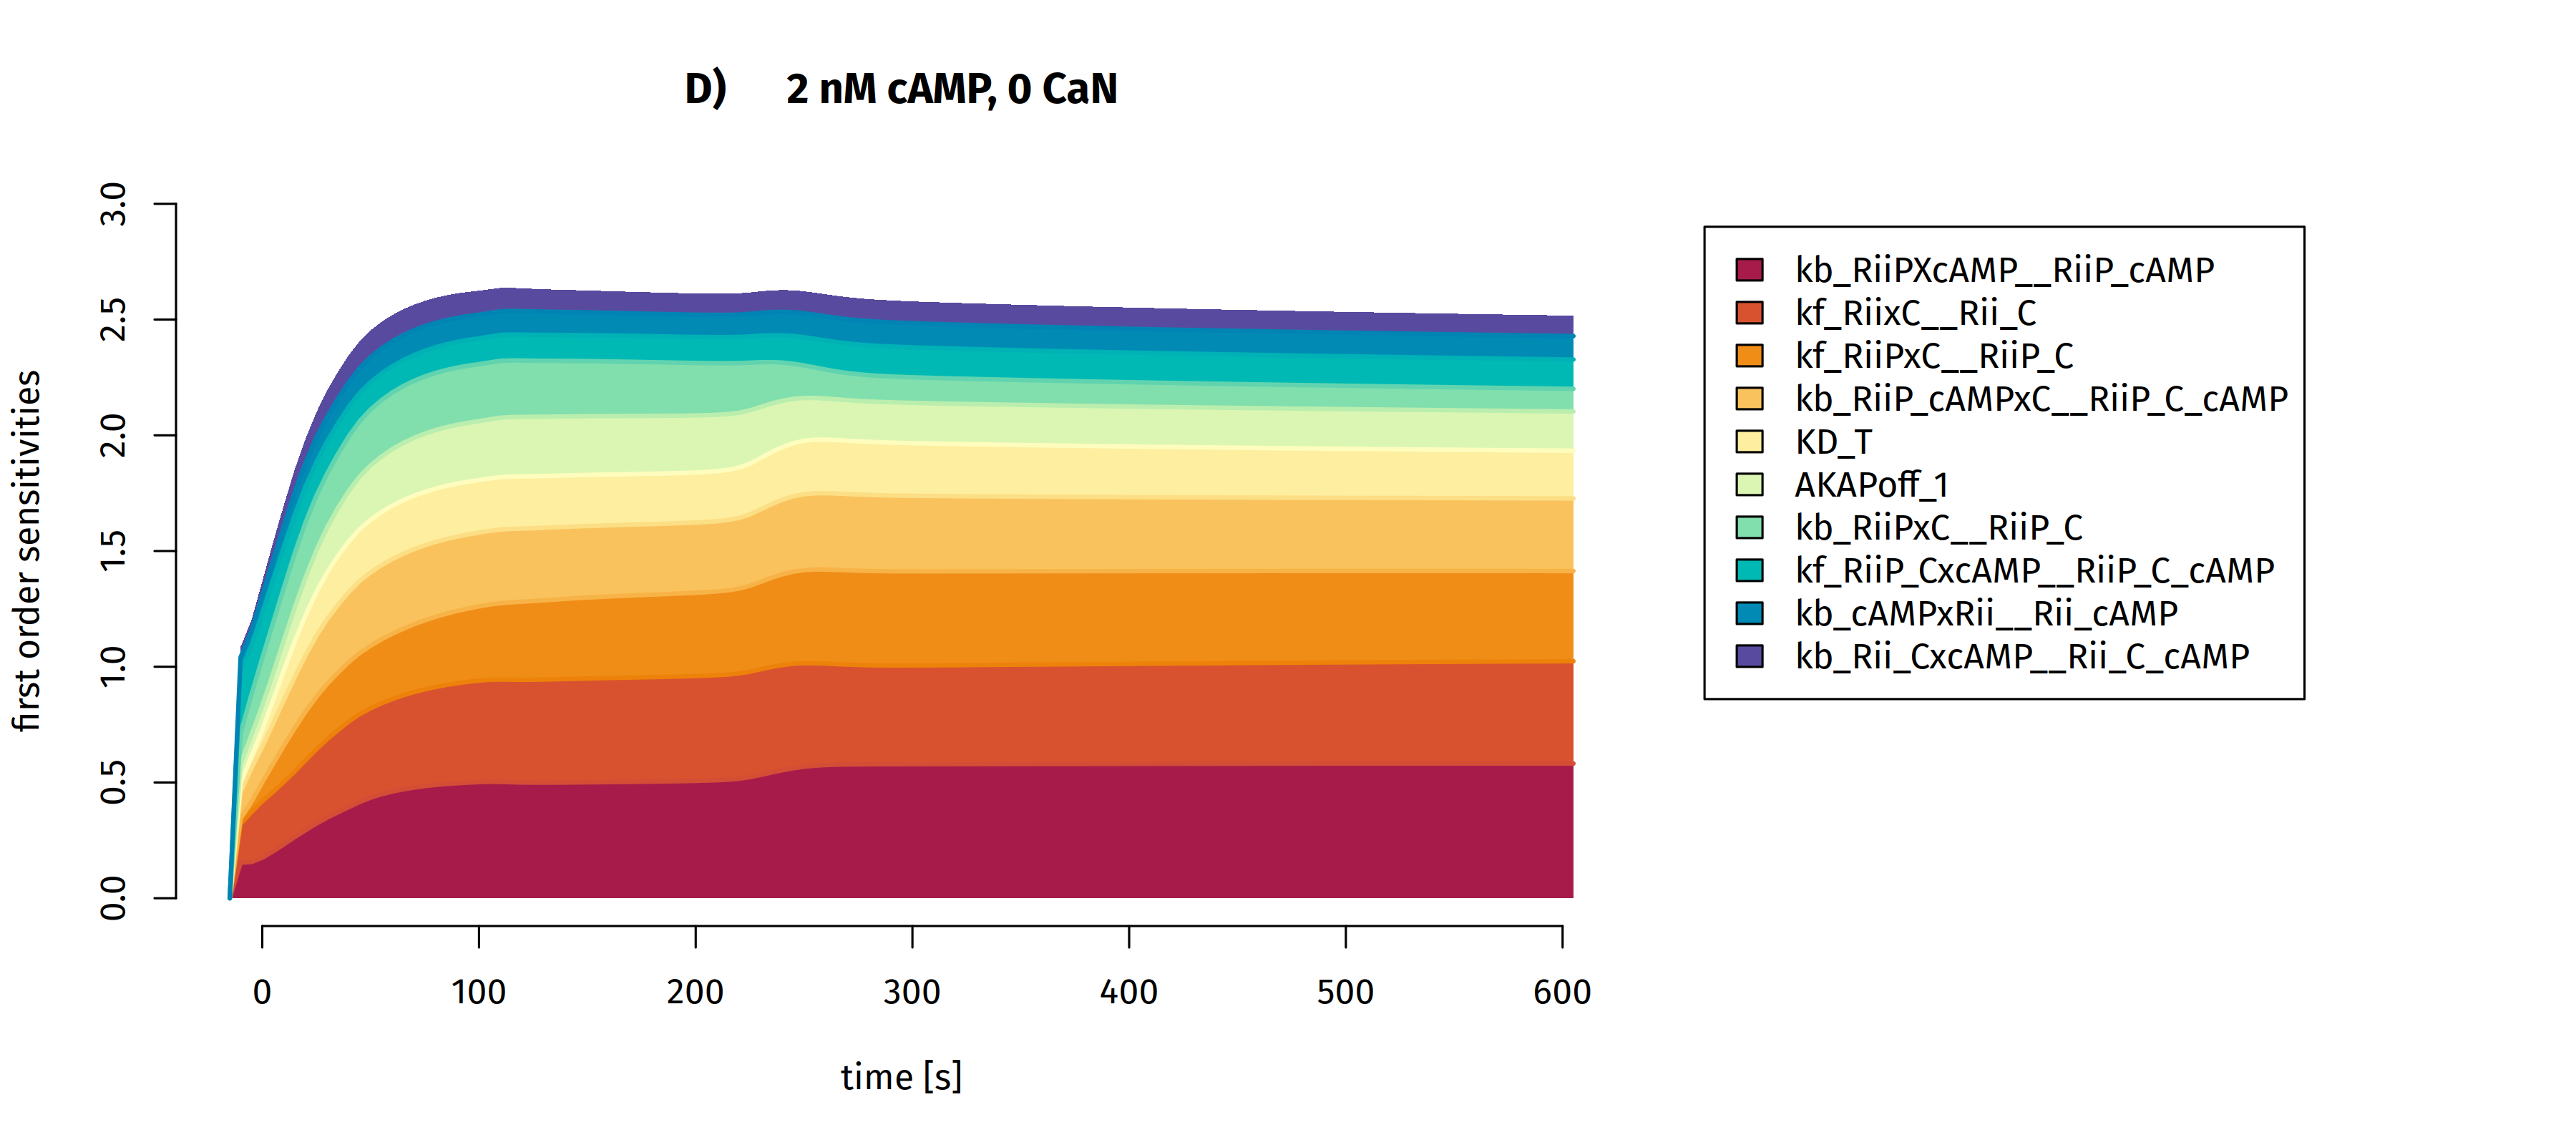}
  \caption{Here we show one of the other pairwise probability density
    panels (A), with a maximum likelihood estimate of the parameters
    (MLE). (B) The trajectories of the observable \texttt{AKAP4p}
    together with the data points. (C) The trajectories of one of the
    state variables (it was not observed in experiments). (D) shows
    the global sensitivity, using the binning method. Included are the
    10 parameters with the largest first order Sobol sensitivity
    indices (others omitted). Knowing the parameter
    \texttt{kb\_RiiPXcAMP\_\_RiiP\_cAMP} would reduce prediction
    uncertainty the most. As predicted value we used one of the state
    variables: \texttt{RiiP\_C}, i.e. phosphorylated \texttt{Rii},
    with bound \texttt{C}.
    \label{fig:AKAP79-state-func-gsa}}
\end{figure}

The simple algorithms, without parallel tempering, produce quite bad
samples, with very big auto-correlations. We had to thin out the raw
sample before estimating the auto-correlation. For Random Walk
Metropolis we obtained a raw sample of size $15 \times 10^6$.

The SMMALA algorithm is more difficult to use than ABC or Random Walk
Metropolis, as it requires more ingredients (more model functions, and
a special simulator that calculates the Fisher information
matrix). For some models, it may be not feasible to use this
algorithm. We recommend using it, when possible, with parallel
tempering (with a reasonable number of different $\beta$
values). The other algorithms also work reasonably well,
and can compensate with a larger raw sample size.

\begin{table}
  \centering
  \begin{tabular}{rrlcc}
    \toprule
    algorithm&sample size $N$&$v$ [$\unit{\per\second}$]&$\tau_{l,\text{int.}}$&Wall Clock time [$\unit{\minute}$]\\
    \midrule
    ABC 14& $11.2 \times 10^3$ & $0.00085(2)$ & $8(4) \times 10^3$& $129$\\
    ABC 120 & $120\times 10^3$ & $0.015(3)$ & $365(79)$ & $180$\\
    RWM& $15.36 \times 10^6$ & $0.16(2)$ & $14(2)\times 10^3$ & $54$ \\
    PT RWM 128 & $120 \times 10^3$ & $0.0014(5)$ & $128(42)\times 10^2$ & $55.2$\\
    PT RMW 16 & $960 \times 10^3$ & $1.30(8)$ & $109(6)$ & $56$\\
    SMMALA & $ 84\times 10^3$ & $0.33(4)$ & $54(6)$ & $39.4$ \\
    PT SMMALA 128 & $80\times 10^3$ & $0.023(3)$ & $72(9)$ & $408.0$\\
    PT SMMALA 16 & $640 \times 10^3$ & $0.89(6)$ & $120(8)$ & $49.7$\\
    \bottomrule
  \end{tabular}
  \caption{This table summarizes the performance of each algorithm on
    a deterministic model with 27 parameters (AKAP79). The performance
    indicator $v$ is the effective sampling speed in points per second
    (higher is better). The measurements were done on one node of
    Dardel, the HPC cluster at KTH. One node has 128 cores. Parallel
    tempering (PT) can split the workload in several different ways,
    we include a split with 128 temperatures, and one with 16
    different temperatures (but still 128 workers, with repeated
    temperatures). For the ABC algorithm, we tried different splits
    between trivial parallelizations of chains and experiments: 120
    parallel Markov chains, versus 14 parallel Markov chains with
    parallel simulation of the 18 available experiments (ODE
    solutions). Abbreviations -- \emph{RWM}: random walk Metropolis,
    \emph{SMMALA}: simplified manifold Metropolis adjusted Langevin
    algorithm; \emph{ABC}: approximate Bayesian computation.\label{tab:benchmark}}
\end{table}

\bibliographystyle{unsrt}

\bibliography{document}

\end{document}
